# Supplementary material for: Efficient nonlinear flame response modeling for propulsion thermoacoustic analysis using limited numerical data
Source: arXiv:2409.05885 source file (2026-08-03)
Supplement: Supplementary file 1 [file Supplementary_Material_pdf.pdf]

## Supplementary Material

---

---

### A. The fundamental neural network used in this work

CNNs are employed in constructing the CNN-embedding module and the Temporal detail module. The reason behind using CNNs for these two modules is their inherent capacity to preserve the temporal order of sequence during feature extraction, it is crucial to use sequence models like LSTM or Transformer to capture chronological features. CNNs achieve this by extracting features through convolutional operations using convolution kernels. As network layers deepen, the sequence length decreases while the feature channel dimension increases. In this study, each convolutional layer within the sequence pyramid employs convolutional kernels of size  $3 \times 1$  and an average pooling window size of  $2 \times 1$ , with a stride of 2 for downsampling. Consequently, after each convolutional and average pooling operation, the sequence length is halved compared to the previous layer and this reduction is especially helpful for training sequence models like LSTM or Transformer, as lengthy input sequences pose challenges for effective training.

Long Short-Term Memory (LSTM) is a sequence model, that can extract temporal and contextual features of sequences, so it is suitable for processing sequence data. Unlike traditional RNN structures, LSTM incorporates cell states and three gate operations, which enable them to effectively address the long-term dependency problem, as illustrated in Fig. S1. The three gate operations are the forget gate, input gate, and output gate. The forget gate takes the previous hidden layer state  $h_{t-1}$  and the current time step information  $x_t$  as inputs. It is computed using the sigmoid activation function (S1), yielding the forget gate activation  $f_t$ .  $f_t$  is then element-wise multiplied with the cell state from the previous time step  $c_{t-1}$ . The initial values of  $c_0$  and  $h_0$  can be obtained through random parameterization or initialization to zero.

$$\sigma(x) = \frac{1}{1 + e^{-x}} \quad (\text{S1})$$

Through computing using the  $\sigma$  function, the values in  $f_t$  are within the range of 0 to 1. When performing element-wise multiplication with  $c_{t-1}$ , the forget gate discards the information from  $c_{t-1}$  corresponding to 0 in  $f_t$ . The larger the value in  $f_t$ , the more information from  $c_{t-1}$  is retained. On the other hand, the information from  $c_{t-1}$  corresponding to 1 in  $f_t$  is preserved entirely. As a result, the forget gate acts as a filter for the information from the previous time step.

Similarly, the input gate serves as a filter for the information at the current time step. The input gate operation consists of two parts. The first part is similar to the forget gate, yielding the input gate activation

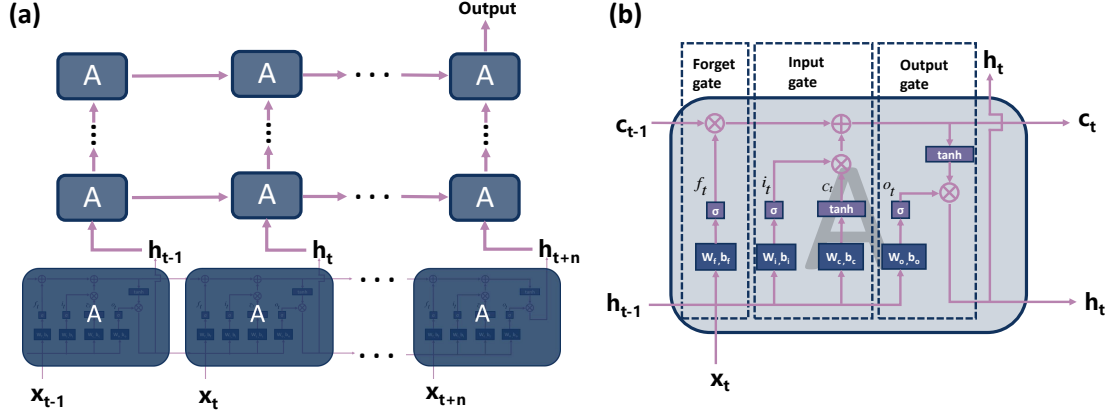

Figure S1: The architecture of the LSTM.

$i_t$ . The second part takes the previous hidden layer state  $h_{t-1}$  and the current time step information  $x_t$  as inputs. These inputs are processed through the activation function  $\tanh$  and element-wise multiplied with  $i_t$  to filter the information at the current time step. Then by adding the output of the forget gate processing, the new cell state  $c_t$  is obtained, which incorporates information from both the previous and current time steps.

Furthermore, by taking  $h_{t-1}$  and  $x_t$  as inputs, the output gate produces  $o_t$ . It utilizes the  $o_t$  to filter information similar to forget and input gate.  $o_t$  is then element-wise multiplied with the  $c_t$  that has been processed by the  $\tanh$  activation function. The result is the hidden state  $h_t$  at the current time step. It is worth mentioning that  $\tanh$  and  $\sigma$  are widely used activation functions in deep learning [1].

All the steps described above, i.e., the processing of the current time step information by the LSTM unit can be described by Fig. S1 (b) and the following equations:

$$\begin{aligned}
 f_t &= \sigma(W_f \cdot [h_{t-1}, x_t] + b_f), \\
 i_t &= \sigma(W_i \cdot [h_{t-1}, x_t] + b_i), \\
 \tilde{c}_t &= \tanh(W_c \cdot [h_{t-1}, x_t] + b_c), \\
 c_t &= f_t \odot c_{t-1} + i_t \odot \tilde{c}_t, \\
 o_t &= \sigma(W_o \cdot [h_{t-1}, x_t] + b_o), \\
 h_t &= o_t \odot \tanh(c_t), \\
 \tanh(x) &= \frac{e^x - e^{-x}}{e^x + e^{-x}},
 \end{aligned} \tag{S2}$$

where  $W_f, W_i, W_c, W_o, b_f, b_i, b_c$ , and  $b_o$  are learnable parameters, and  $\odot$  denotes the element-wise multiplication operation.

Long Short-Term Memory (LSTM) is a recurrent neural network known for its sequential processing of input sequence features, specifically the computation at time step  $t_n$  relies on the hidden layer state at time step  $t_{n-1}$ . Consequently, LSTM inherently operates sequentially within training examples, making

parallelization challenging. Moreover, LSTM with gradient vanishing issues and struggles with capturing long-term dependencies in exceeding long input sequences [2, 3]. On the contrary, the Transformer model is well-suited for handling sequence data with long-term dependencies. Its attention mechanism enables efficient information interactions between different time steps within the sequence, which performs excellent information extraction capabilities [4].

The Transformer model comprises two main parts: the encoder and the decoder. In this study, only the encoder part is utilized for sequence information extraction, the encoder contains N layers encoder layer as shown in Fig. S2 (a). We construct the Encoder module in our study using the single encoder layer of the Transformer. The encoder layer primarily consists of a multi-head attention module and a position-wise Feedforward Network (FFN) module. To enhance network depth and facilitate more efficient training, residual connections [5] and Layer Normalization [6] are incorporated. The overall architecture of the Encoder module is depicted in Fig. S2 (b).

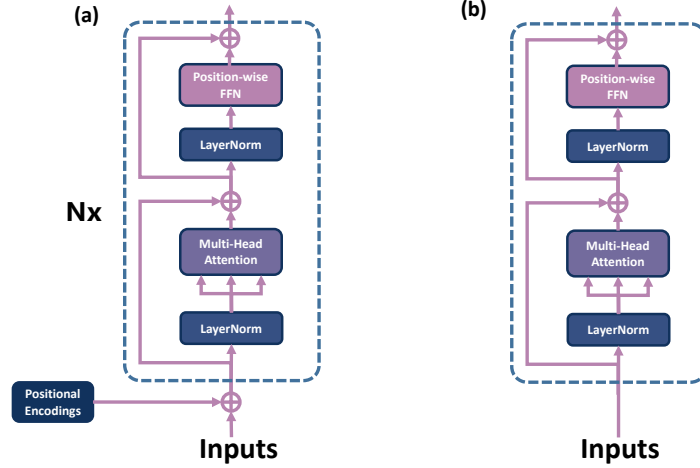

Figure S2: (a) The architecture of the Transformer encoder. (b) The architecture of the Encoder module used in this study.

The core of the Transformer model is its attention mechanism (similarly, the Injector module is also constructed using the attention mechanism). Therefore, this discussion will focus primarily on the attention mechanism, while more comprehensive details about Transformer can be found in the original work by Vaswani et al. [4]. The attention mechanism comprises three main components: queries, keys, and values, as depicted in Fig.3(d). These components are denoted as follows: queries ( $Q \in \mathbf{R}^{N_q, D_q}$ ), keys ( $K \in \mathbf{R}^{N_k, D_k}$ ), and values ( $V \in \mathbf{R}^{N_v, D_v}$ ). The attention operation can be computed using the following equations:

$$\begin{aligned} \mathcal{A}_{sc}(Q, K, V) &= \mathcal{S}_{max} \left( \frac{QK^T}{\sqrt{D_k}} \right) \\ \mathcal{A}(Q, K, V) &= \mathcal{S}_{max} \left( \frac{QK^T}{\sqrt{D_k}} \right) V \\ \mathcal{S}_{max}(x_i) &= \frac{e^{x_i}}{\sum_{i=1}^n e^{x_i}} \end{aligned} \quad (S3)$$

In the equations,  $N_q$  denotes the sequence length of queries, while  $N_k$  denotes the sequence length of keys

and values (keys and values having the same length).  $D_q$  denotes the feature dimension of queries and keys (which must be identical), and  $D_v$  denotes the feature dimension of values. The term  $\mathcal{A}_{sc}(Q, K, V)$  denotes the attention score matrix. The *softmax* function ( $\mathcal{S}_{max}$ ) is applied row-wise to the attention score matrix and scaled by  $\sqrt{D_k}$  to mitigate the issue of gradient vanishing caused by *softmax* function [4]. Rather than employing single-head attention, the Transformer model utilizes multi-head attention  $\mathcal{A}_{mh}$ . The original features  $Q, K, V$  are first transformed through three separate fully connected layers, resulting in feature dimensions of  $D_q, D_q, D_v$ , respectively. Subsequently, these dimensions are divided by  $H$ , which denotes the number of attention heads. Consequently, each attention head possesses feature dimensions of  $D_q/H$ . The attention operation is performed similarly for each head. Finally, the dimensions  $D_q$  are constructed by concatenating (defined as  $\mathcal{C}_c$  in Eq. (S4)) the outputs from each attention head. The computations involved in multi-head attention  $\mathcal{A}_{mh}$  are illustrated in the subsequent equations:

$$\begin{aligned}\mathcal{A}_{mh}(Q, K, V) &= \mathcal{C}_c(head_1, \dots, head_H)W^o \\ head_i &= \mathcal{A}(QW_i^q, KW_i^k, VW_i^v)\end{aligned}\tag{S4}$$

where  $W_i^q, W_i^k, W_i^v$  are learnable parameters of fully connected layers of  $i$ th head. It is important to note the distinction between two types of attention mechanisms based on the source of input features. When the queries, keys, and values all originate from the same set of input features, this configuration is referred to as self-attention. Conversely, when they derive from different input features, we refer to the mechanism as cross-attention. For example, in the case of the multi-head attention used in the Encoder and Injector modules of some architectures, the mechanism functions as cross-attention.

## B. Chronological Feature Path (CFP)

Chronological features play a pivotal role in the precise construction of a flame response, as evident in Supplementary Material D. In our investigation, we conduct a comparative analysis of the Transformer architecture with and without chronological information. Our findings demonstrate that the Transformer equipped with chronological information excels in constructing an accurate flame nonlinear response, while the absence of chronological information has no this capability. Consequently, we have devised a CFP to facilitate the extraction of chronological features. Within this path, the Long Short-Term Memory (LSTM) layers are responsible for the task of extracting the chronological features. However, direct input of the original sequence into LSTM is impractical, as it poses challenges to the effective training of LSTM. To address this issue, we have introduced a CNN-embedding module. This module comprises four convolutional layers, with each convolutional layer halving the sequence length while increasing the feature dimension at each instance. Specifically, in this study, the first convolutional layer of the CNN-embedding module increases the dimension by 32, followed by dimensions of 64, 128, and 128 for the second, third, and fourth layers, respectively. This module is for reducing the sequence length while preserving the inherent chronological

order of the sequence. So it can address the purpose of sequence length reduction without sacrificing the chronological information of the data, thereby facilitating the subsequent tasks of chronological feature extraction within the LSTM layers.

### C. Temporal Detail Feature Path (TDFP)

In the context of flame nonlinear response modeling, the sensitivity of the neural network model to changes in the velocity perturbations value at each instance or changes in the chronological order of instances plays a pivotal role in accurately constructing the flame nonlinear response. Consequently, the neural network must exhibit sensitivity to such changes to effectively capture corresponding changes in the output heat release rate. To achieve this, low-level features, which closely the original input features and include more detailed information about the input sequence, are employed. These features are closer to the input layer of a neural network and it will be abstracted and integrated into high-level features in the process of network forward propagation. Some studies have identified an "information bottleneck" phenomenon in the propagation process of neural networks [7, 8]. During forward propagation, the network often compresses or discards detailed information, resulting in a tendency to learn low-frequency mapping relationships that may overlook finer details [9, 10]. So the higher-level features that are closer to the output layer tend to lose detailed information. In the context of constructing the flame nonlinear response, we believe that the detailed temporal information inherent in low-level features is indispensable for sensitively capturing changes in the flame response, thereby enhancing the accuracy of construction. Therefore, we introduce a TDFP to facilitate the model's capture of temporal details.

The TDFP comprises a Temporal detail module and two Encoder modules. Differing from the CFP, we sample the original sequence as a short sequence using the sparse-to-dense sampling method outlined in Sec.5. This short sequence incorporates prior information about the flame's response, enhancing the precision of the flame nonlinear response construction. The Temporal detail module is responsible for conducting shallow learning of the input short sequence, so it just consists of only two layers of CNN. The limited number of CNN layers ensures that the module can output a longer sequence while retaining more detailed information during feature extraction. In contrast, the CNN-embedding module in the CFP includes four CNN layers, resulting in an output sequence length four times short of the Temporal detail module. The Injector module serves to facilitate feature interaction between the two paths by injecting temporal detail features into the CFP. This interaction enables the Long Short-Term Memory (LSTM) component to access more detailed temporal information for improved construction of the flame nonlinear response. The Injector module is composed of a cross-attention mechanism, where queries are obtained from the CFP, while keys and values are from the TDFP. This attention mechanism has powerful feature-extraction capabilities, extracting suitable features from values based on queries. Thus, it extracts appropriate features from the TDFP based on the CFP. Additionally, we incorporate learnable parameters  $\alpha_i \in \mathbf{R}^D$  ( $D$  representing

feature dimensions of  $F_{Injector_i}$ ) to control the proportions of temporal detail features injected into the CFP, as illustrated in Eq. (S5).

$$\begin{aligned}\hat{F}_{CN} &= F_{CN} + \alpha_1 F_{Injector_1} \\ \hat{F}_{LSTM_2} &= F_{LSTM_2} + \alpha_2 F_{Injector_2}\end{aligned}\tag{S5}$$

where  $\alpha_i$  is initialized by a standard normal distribution.  $F_{CN}$  denotes the features output from CNN-embedding module,  $F_{LSTM_2}$  denotes the features output from  $LSTM_2$  layers.  $F_{Injector_1}$  and  $F_{Injector_2}$  denote features output from Injector1 module and Injector2 module respectively, as shown in Fig.3(a).

The Encoder module adopts the architecture of the Transformer encoder layer, as depicted in Fig. S2 (b). However, it is different from the typical Transformer encoder layer by employing cross-attention rather than self-attention. In this cross-attention, queries are from the TDFP, while keys and values are from the CFP. This module plays the role of updating temporal detail features to produce greater diversity and richness of temporal detail features across the entire neural network model. The LSTM-processed features carry substantial contextual information of input sequence, representing the neural network model’s understanding of flame nonlinear response. Consequently, we employ these features as both keys and values within the Encoder module to enhance the temporal detail features. This approach ensures that the updated temporal detail features align closely with the features relevant to a flame nonlinear response. Our tests have proved the efficacy of the TDFP in our model. As demonstrated in Supplementary Material B, our model, equipped with the TDFP, exhibits superior generalization capabilities when compared to the Single-Path model.

#### D. The importance of chronological features

In this section, we have devised a Single-Path neural network architecture, as illustrated in Fig. S3. We choose the Transformer encoder as the sequence model, primarily due to the ease of peeling the positional encoding module from the Transformer framework. This module serves a critical role in infusing chronological information into the Transformer model. Without it, the Transformer struggles to extract chronological features effectively, primarily due to the inherent spatial replacement invariance of the attention mechanism, as explained in Vaswani et al.’s seminal work on attention mechanisms [4]. Fig. S4 provides a comparative analysis of the performance of the Single-Path model equipped with positional encoding (with chronological information) and without positional encoding (lacking chronological information). The results show that capturing chronological features is important to constructing flame nonlinear responses, particularly at lower frequencies.

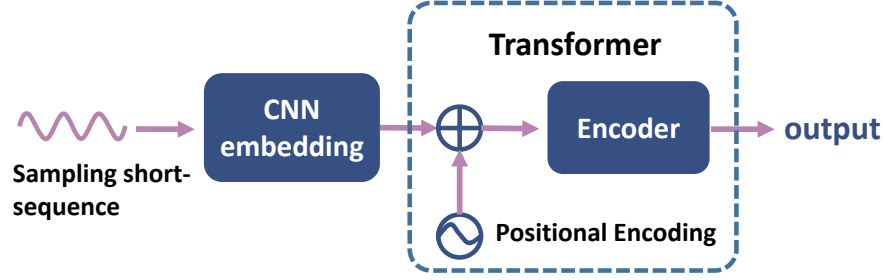

Figure S3: The schematic of the Single-Path model using Transformer.

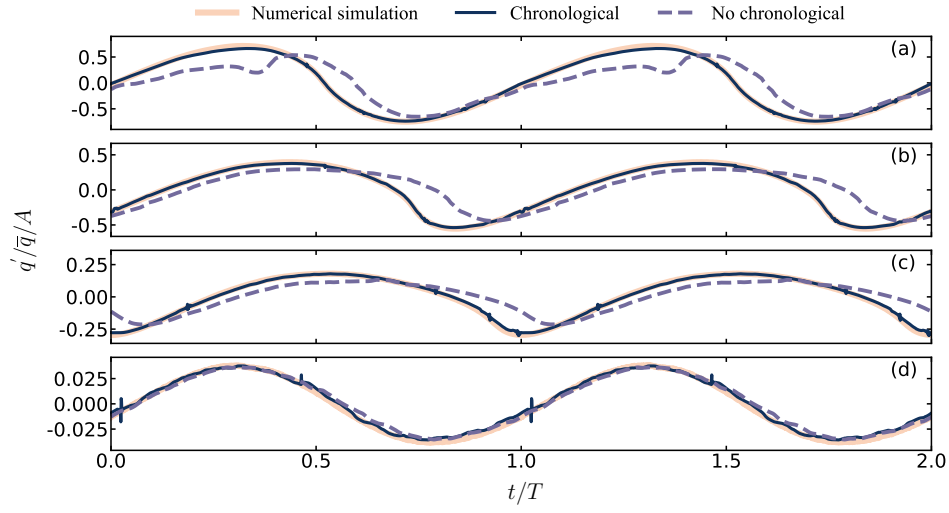

Figure S4: Comparison of predicted results with (blue solid lines) and without (purple dashed lines) chronological information.  $A = 0.55$ , and the frequencies from (a) to (d) are 200 Hz, 300 Hz, 400 Hz, and 800 Hz. The original input sequence length  $n$  is 6000, and the short sequence sampling length  $n_s$  is set to 1000. Orange solid lines: numerical simulation results.

### E. The generalization capability of Dual-Path model

In this section, we have shown the generalization capabilities of the Dual-Path model by conducting a comparative analysis with the Single-Path model under two special data distributions. The two data distributions are as follows: firstly, the special nonlinearity observed in the 510 Hz to 660 Hz frequency range, as detailed in Sec.6.2; secondly, the deviation in data values of SAHF signals. The Single-Path model, depicted in Fig. S5, comprises only a Chronological Feature Path (CFP) and has no Temporal Detail Feature Path (TDFP). To evaluate the models, we present the prediction results for both the Single-Path and Dual-Path models in Fig. S6 for frequencies within the 510 Hz to 660 Hz range. The results show the better performance of the Dual-Path model over the Single-Path model. Furthermore, we evaluate the predictive capabilities of both models for SAHF signals, as shown in Fig. S7. The Single-Path model exhibits poor predictive performance, even failing to predict well for an amplitude of 0.25. In contrast, the Dual-Path model demonstrates its ability to predict the response of SAHF signals. These results prove that TDFP can enhance the generalization capabilities of the model.

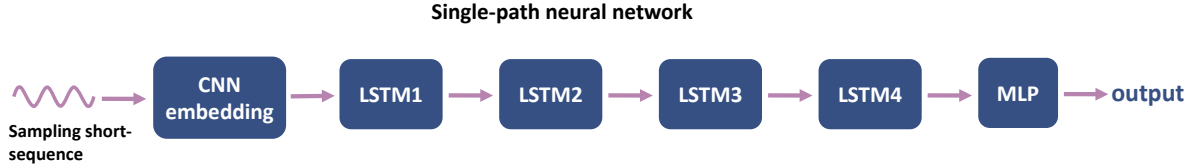

Figure S5: The schematic of Single-Path-model using LSTMs.

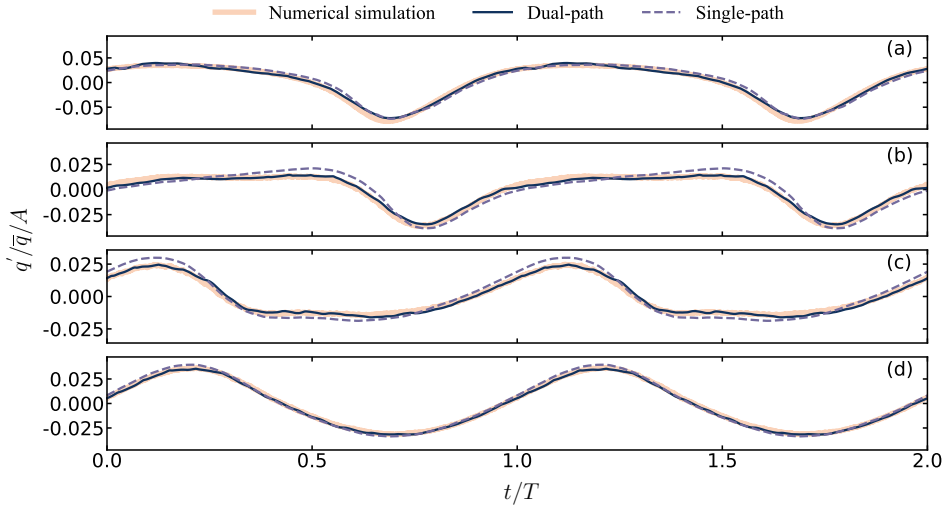

Figure S6: Comparison of predicted results between Single-Path (purple dashed lines) and Dual-Path model (blue solid lines) for special data distribution of 510 to 660 Hz.  $A = 0.55$ , and the frequencies from (a) to (d) are 510 Hz, 550 Hz, 600 Hz, and 660 Hz.  $n = 6000$ , and  $n_s = 1000$ .

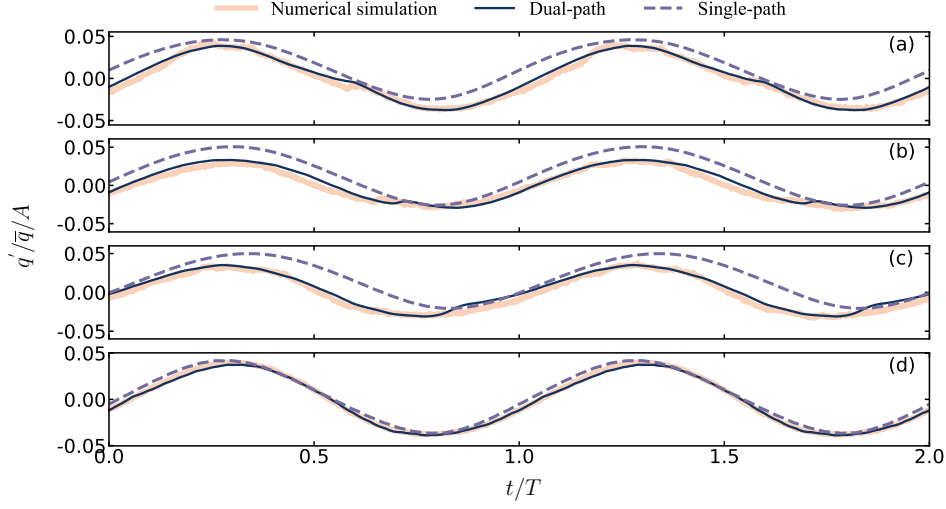

Figure S7: Comparison of prediction results between Single-Path (purple dashed lines) and Dual-Path model (blue solid lines) for SAHF signals. From (a) to (c), the frequencies are 700 Hz, 800 Hz, and 900 Hz respectively, and  $A = 0.1$ . For (d),  $f = 800$  Hz and  $A = 0.25$ .  $n = 6000$ , and  $n_s = 1000$ .

## F. Construction capability of flame nonlinear response without special data distribution in frequency

The inlet steady-state velocity of the numerical simulation is set at 1 m/s in Sec.2, which has performed special data distribution in the frequencies 510 to 660 Hz. In this section, we set the inlet steady-state velocity at 0.6 m/s, which does not perform special data distribution at any frequency. Fig. S8 shows the predicted results of the inlet steady-state velocity setting at 0.6 m/s. These results show that the MRE of different frequencies are all under 5%, therefore, it proves that our method can predict the flame nonlinear response at any frequency with high precision.

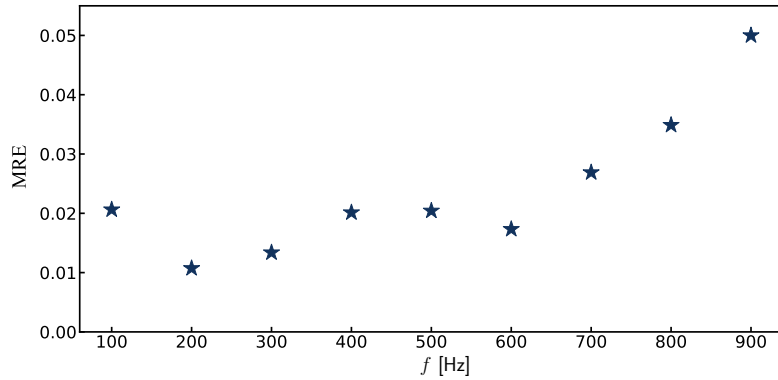

Figure S8: The predicted results of steady-state velocity setting at 0.6 m/s.  $A = 0.55$ , and frequencies are 100 to 900 Hz with a step of 100 Hz.

### G. Transfer learning capability of the Dual-Path model for SAHF signals

This section explores the transfer learning capabilities of the Dual-Path model when applied to Small-Amplitude High-Frequency (SAHF) signals. Initially, the model is trained using the 0.5 s dataset described in Sec.3. Subsequently, all parameters except for the MLP module are frozen, and the MLP module alone is fine-tuned. This study utilizes two short-duration SAHF signals with different frequencies for fine-tuning, enhancing the model's prediction accuracy across a spectrum of frequencies. Specifically, we fine-tune the model using two 0.01 s signals at frequencies of 800 Hz and 900 Hz, each with an amplitude of 0.1.

Fig.S9 presents the time-domain prediction results for single-frequency signals with and without the fine-tuning process. Additionally, Fig.S10 displays the Mean Relative Error (MRE) for various frequencies within the 800 to 900 Hz range. The fine-tuned model demonstrates superior performance, particularly at frequencies such as 810 Hz, 820 Hz, 880 Hz, and 890 Hz, which are proximal to the two base training frequencies of 800 Hz and 900 Hz. These findings suggest that employing more short-duration SAHF signals (three or four) for fine-tuning could further enhance the Dual-Path model's predictive accuracy for SAHF signals.

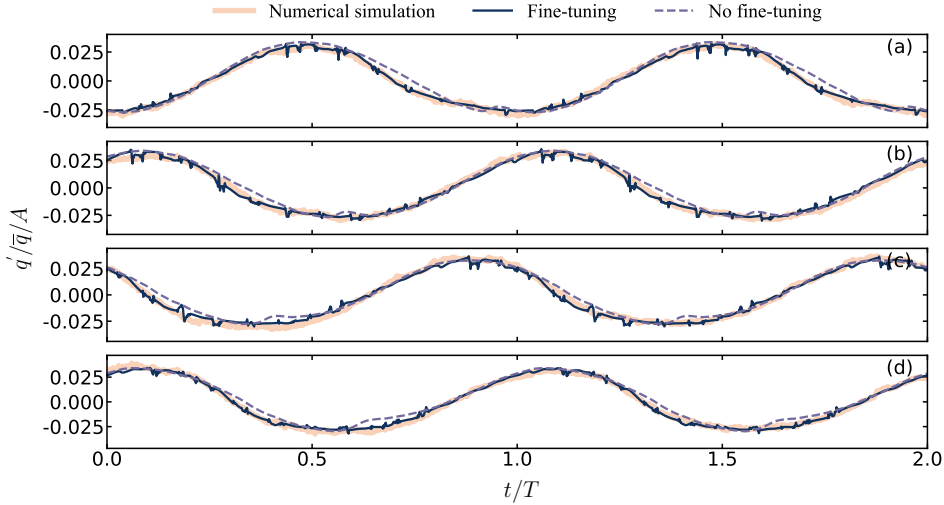

Figure S9: Comparison of prediction results between without (purple dashed lines) and with fine-tuning (blue solid lines).  $A = 0.1$ , and the frequencies from (a) to (d) are 820 Hz, 840 Hz, 860 Hz, and 880 Hz.  $n = 6000$ , and  $n_s = 1000$ .

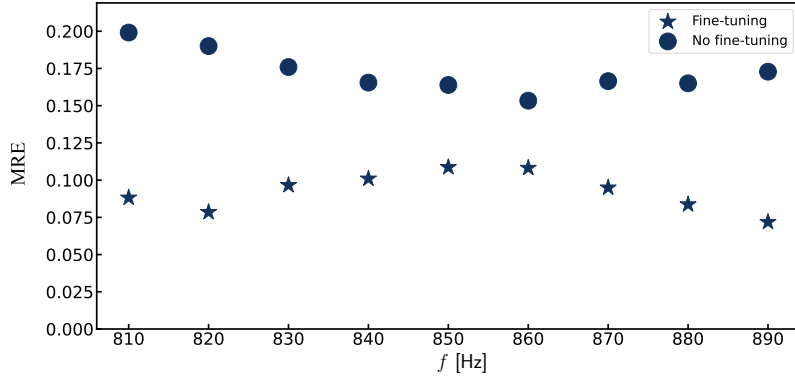

Figure S10: The comparison of predicted results of fine-tuning and without fine-tuning.  $A = 0.1$ , and the frequencies are from 810 to 890 Hz with a step of 10 Hz.

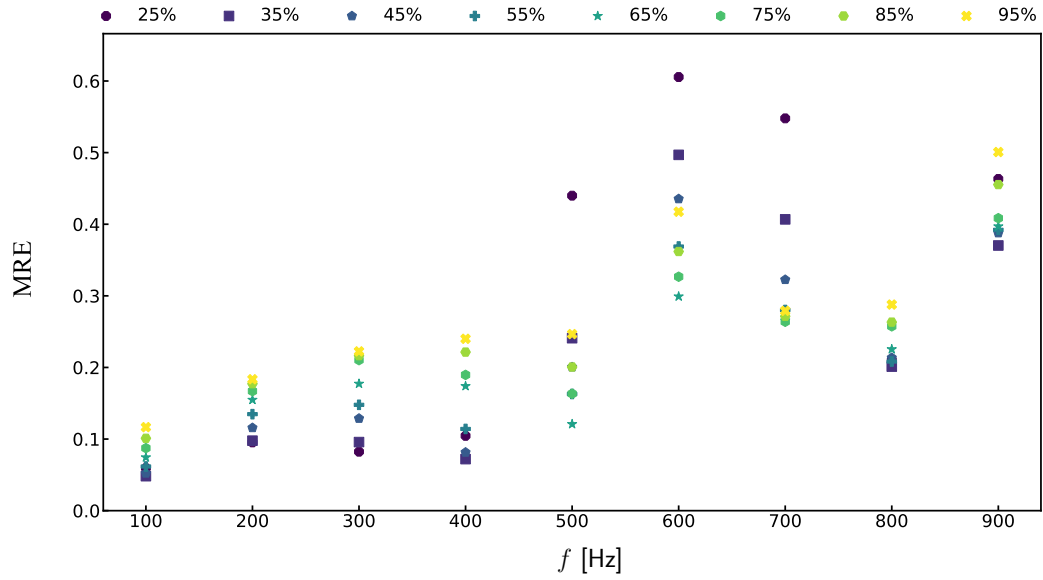

Figure S11: The MRE of single-frequency signals of MLP with different amplitudes ( $A$  equals the value after the marker at the top of the figure) and frequencies.

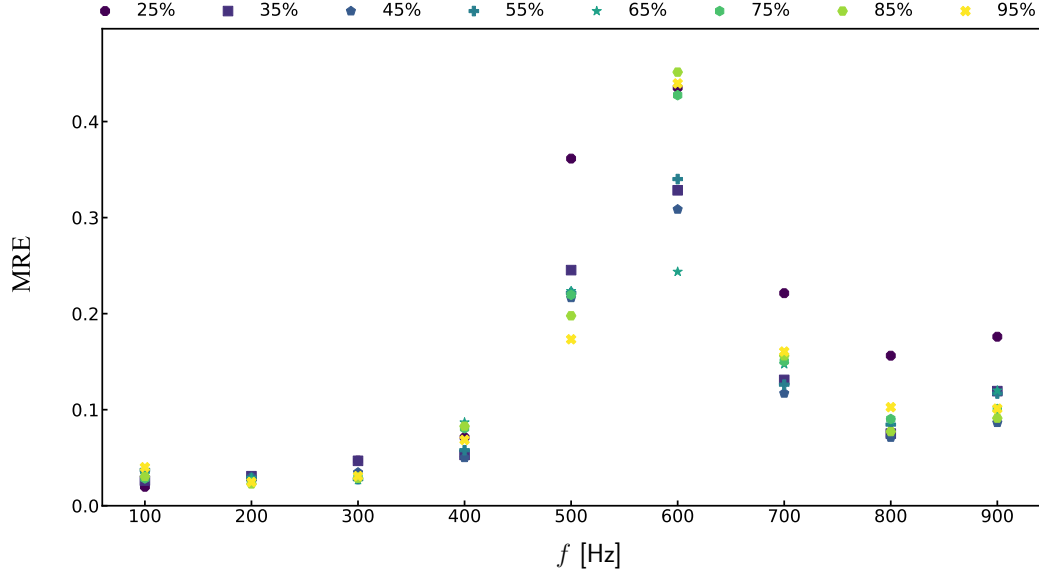

Figure S12: The MRE of single-frequency signals of LSTM with different amplitudes ( $A$  equals the value after the marker at the top of the figure) and frequencies.

## References

- [1] S. R. Dubey, S. K. Singh, B. B. Chaudhuri, Activation functions in deep learning: A comprehensive survey and benchmark, *Neurocomputing* (2022).
- [2] S. Hochreiter, The vanishing gradient problem during learning recurrent neural nets and problem solutions, *Int. J. Uncertain. Fuzziness Knowledge-Based Syst* 6 (1998) 107–116.
- [3] Y. Bengio, P. Simard, P. Frasconi, Learning long-term dependencies with gradient descent is difficult, *Int. J. Neural Netw* 5 (1994) 157–166.
- [4] A. Vaswani, N. Shazeer, N. Parmar, J. Uszkoreit, L. Jones, A. N. Gomez, L. Kaiser, I. Polosukhin, Attention is all you need, *Adv. Neural Inf. Process. Syst* 30 (2017).
- [5] K. He, X. Zhang, S. Ren, J. Sun, Deep residual learning for image recognition, in: *Proc. IEEE Int. Conf. Comput.*, 2016, pp. 770–778.
- [6] J. L. Ba, J. R. Kiros, G. E. Hinton, Layer normalization, *arXiv preprint arXiv:1607.06450* (2016).
- [7] N. Tishby, F. C. Pereira, W. Bialek, The information bottleneck method, *arXiv preprint physics/0004057* (2000).
- [8] N. Tishby, N. Zaslavsky, Deep learning and the information bottleneck principle, in: *IEEE Int. Symp. IEEE*, 2015, pp. 1–5.
- [9] Z. Liu, W. Cai, Z.-Q. J. Xu, Multi-scale deep neural network (mscalednn) for solving poisson-boltzmann equation in complex domains, *arXiv preprint arXiv:2007.11207* (2020).
- [10] X.-A. Li, Z.-Q. J. Xu, L. Zhang, Subspace decomposition based dnn algorithm for elliptic type multi-scale pdes, *J. Comput. Phys* 488 (2023) 112242.
